# Supplementary material for: NoWag: A Unified Framework for Shape Preserving Compression of Large Language Models
Source: arXiv:2504.14569 source file (2026-01-27)
Supplement: Supplementary file 1 [file Normalization.tex]

%figs needed
%distribution fig

%
\section{Effect of Normalization on Weights}
\label{app:Normalization}
% \red{
% TODOs:
% \begin{itemize}
%     \item add colorbar to Fig 2
%     \item add 
% \end{itemize}
% }
Below are two plots illustrating the effects of normalization has on the weights. For both plots, we used the weights of the Q projection of the first layer of the Llama 2 7B parameter model. In figure \ref{fig:weight_plot}, we plot out the weights before and after normalization, and in figure \ref{fig:weight_distribution} we plot out the distribution of the consecutive groups of 6 elements that we quantized together with \methodVQ.
\input{Figs/weight_dist}
\begin{figure}[H]
    \centering
    \includegraphics[width=0.9\linewidth]{"Figs/layer_0-self_attn.q_proj_weights.png"}
    \caption{Left, plot of the original weight matrix without normalization, right the plot of the normalized weight, columns and rows with large norms have been broken up}
    \label{fig:weight_plota}
\end{figure}
\subsection{Effect of Normalization On Sparsity}
Below, we examine the effects of the normalization on the resulting locations of the pruned weights. Empirically, as shown in in figures \ref{fig:weight_distributiona} and \ref{fig:weight_plota}, normalization appears to have a similar impact as output group based pruning.
\begin{figure}[H]
    \centering
    \includegraphics[width=\linewidth]{Figs/layer_0-self_attn.q_proj_unstructured.png}
    \caption{Plot of the masks of pruned and unprunded elements with Wanda without grouping (left), with grouping (center) and with \methodP (right), for 50$\%$ unstructured pruning, \red{Black} is the preserved elements, white is the pruned.}
    \label{fig:weight_distribution}
\end{figure}
\begin{figure}[tb]
    \centering
    \includegraphics[width=0.9\linewidth]{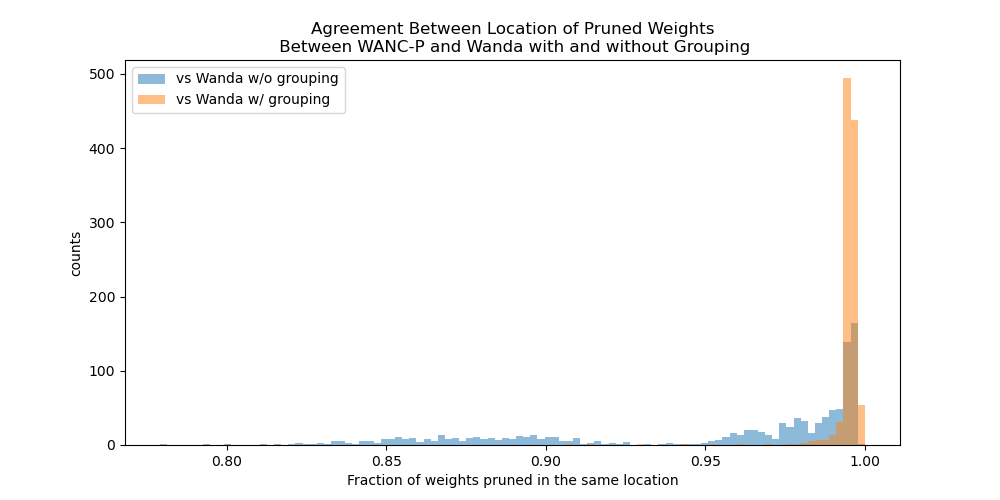}
    \caption{Histogram of the per Layer relative agreement in pruning location between \methodP and Wanda without (blue) and with output group pruning (orange). Calibration dataset for all was 128 samples of RedPajamas. Our Normalization behaves similarly to output group based pruning.}
    \label{fig:weight_distribution}
\end{figure}
